# Supplementary material for: Optimizing Experimental Parameters for Orbital Mapping
Source: arXiv:2305.16039 source file (2023-05-25)
Supplement: Supplementary file 1 [file appendix.tex]

\appendix
\section{}
We present the set of parameters used to calculate the reference images for all systems investigated in this work.

\begin{table}
\begin{center}
\caption{Parameters of the STEM reference image calculations.}
\begin{tabular}{ |m{3cm}|>{\centering\arraybackslash}m{0.9cm}|>{\centering\arraybackslash}m{1.15cm}|>{\centering\arraybackslash}m{1cm} | }
 \hline
STEM & rutile & graphite & STO-LMO\\
 \hline
 thickness (1 unit cell) [\AA{}] & 3 & 4.3 & 7.8\\
 \hline
 step size x [\AA{}] & 0.14 & 0.15 & 0.36\\
 step size y [\AA{}] & 0.14 & 0.21 & 0.24\\
 \hline
 acceleration voltage [kV] & 300 & 60 & 300\\
 \hline
 convergence semi-angle $\alpha$ [mrad] & 30 & 30 & 30\\
 \hline 
 collection semi-angle $\beta$ [mrad] & 50 & 50 & 50\\
 \hline
\end{tabular}
\end{center}

\label{table_STEM}
\end{table}

\begin{table}
\begin{center}
\caption{Parameters of the EFTEM reference image calculations.}
\begin{tabular}{ |m{3cm}|>{\centering\arraybackslash}m{0.9cm}|>{\centering\arraybackslash}m{1.15cm}|>{\centering\arraybackslash}m{1cm} | }
 \hline
EFTEM & rutile & graphite & STO-LMO\\
 \hline
 thickness (1 unit cell) [\AA{}] & 3 & 4.3 & 7.8\\
 \hline
 calibration x [\AA{}/px] & 0.14 & 0.15 & 0.36\\
 calibration y [\AA{}/px] & 0.14 & 0.21 & 0.24\\
 \hline
 acceleration voltage [kV] & 300 & 60 & 300\\
 \hline
 collection semi-angle $\beta$ [mrad] & 46 & 77 & 36\\
 \hline
\end{tabular}
\end{center}

\label{table_EFTEM}
\end{table}
